# Supplementary material for: ADMM-MCBF-LCA: A Layered Control Architecture for Safe Real-Time Navigation
Source: arXiv:2503.02208 source file (2025-03-07)
Supplement: Supplementary file 1 [file 7-Appendix.tex]

\section{Appendix}\label{sec:appendix}
\subsection{Details of 2DOF controller derivation}
% In the next section, we prove that the controllers optimized from running ADMM results in the global exponential stability of the overall closed loop system at convergence for linear systems and asymptotic stability for nonlinear systems.

\textbf{Locally optimal feedback control law}:
From the convergence guarantees of iLQR~\cite{todorov2005generalized}, we have that the feedback control layer in~\eqref{eq:nonlin-track-layer} results in a controller that is locally optimal for each initialization from ADMM solution. Therefore, at every ADMM iteration $k$, the feasibility problem~\eqref{eq:trajectory-gen} is solved once, the controller synthesis problem in~\eqref{eq:fb-control} is approximated by~\eqref{eq:nonlin-track-layer} and solved until iLQR converges followed by the dual update in~\eqref{eq:dual-update}.

Consider the solution to problem~\eqref{eq:nonlin-track-layer} once ADMM has converged and a cost-to-go function of the form
\begin{equation}
    V_{i, p}(\delta x_{i, p}) = \frac{1}{2} \delta x_{i, p}^\top P_{i, p} \delta x_{i, p} + b_{i, p}^\top \delta x_{i, p} + q_{i, p}
\end{equation}
where $P_{i, p} \in \R^{n(N+1) \times n(N+1)}, b_{i, p} \in \R^{n(N+1)}, q_{i, p} \in \R$. The terminal cost for the iterative linear controller is obtained by setting $P_T^{k} = (\rho/2)I, b_T^{k} = \rho c_T^{k}, q_T^{k} = (\rho/2) \| c_T^{k+1} \|_2^2$. Solving via dynamic programming, we get
\begin{equation*}
    V_{i, p}^\star(\delta x_{i, p}^\star) = \min_{\delta u_{i, p}} \frac{\rho}{2} \left\| \begin{bmatrix}
        \delta x_{i, p} + c_{i, p} \\
        \delta u_{i, p} + d_{i, p}
    \end{bmatrix} \right\|_2^2 + V_{i+1}^\star(\delta x_{i+1})
\end{equation*}
where $c_{i, p} = (x_{i, p} - r_{i, p} + v_{r, i})$ and $d_{i, p} = (u_{i, p} - a_{i, p} + v_{a,i})$. The minimizer is given by 
\begin{equation*}
    \delta u_{i, p}^\star = -K_{i, p}^\star \delta x_{i, p} - w_{i, p}^\star
\end{equation*}
where $w_{i, p}^\star = \Phi_{i, p}^{-1} (\rho d_{i, p} + B_{i, p}^{\star\top} b_{i+1})$, $\Phi_{i, p} = Q + B_{i, p}^{\star\top} P_{i+1} B_{i, p}^\star$ with $Q = (\rho/2) I$, and the feedback gain matrix is given by $K_{i, p}^\star = \Phi_{i, p}^{-1}B_{i, p}^{\star\top}P_{i+1^\star}A_{i, p}^\star$.

Plugging $\delta u_{i, p}^\star$ into the cost-to-go function, setting $R = (\rho/2) I$ and simplifying further, we observe the following recursions for the cost weight matrices
\begin{align}
    P_{i, p} &= Q + K_{i, p}^{\star\top}RK_{i, p}^\star + \Bar{A}_{i,p}^{\star\top} P_{i+1}^\star\Bar{A}_{i, p}^\star \\
    b_{i, p}^\star &= \rho K_{i, p}^{\star\top} (w_{i, p}^\star - d_{i, p}^\star) - \Bar{A}_{i, p}^{\star\top} (P_{i+1}^\star B_{i, p}^\star w_{i, p}^\star+ b_{i+1}^\star) + \rho c_{i, p}^\star \\
    q_{i, p}^\star &= \frac{\rho}{2} \left\|\begin{bmatrix}
        c_{i, p}^\star \\
        w_{i, p}^\star \\
        d_{i, p}^\star
    \end{bmatrix} \right\|_2^2 + \frac{1}{2} \| B_{i,p}^\star w_{i, p}^{\star} \|^2_{P_{i+1}^\star} + b_{i+1}^{\star\top} B_{i, p}^\star w_{i, p}^\star + q_{i+1}
\end{align}
where $P_{i, p}^\star$ follow the usual DARE recursion and $\Bar{A}_{i, p}^\star = (A_{i, p}^\star - B_{i, p}^\star K_{i, p}^\star)$. Therefore, the locally optimal control law for each nominal controller $p$ is governed by a feedforward term and a feedback term as
\begin{equation}
    \mu_p^\star(i) := u_{i, p}^\star - w_{i, p}^\star - K_{i, p}^\star \delta x_{i, p}^\star.
\end{equation}
